# Supplementary material for: Multi-View Representation is What You Need for Point-Cloud Pre-Training
Source: arXiv:2306.02558 source file (2024-04-28)
Supplement: Supplementary file 2 [file supp_cotr_2.tex]

\begin{figure}[h]
    \begin{center}
    \includegraphics[width=1\linewidth]{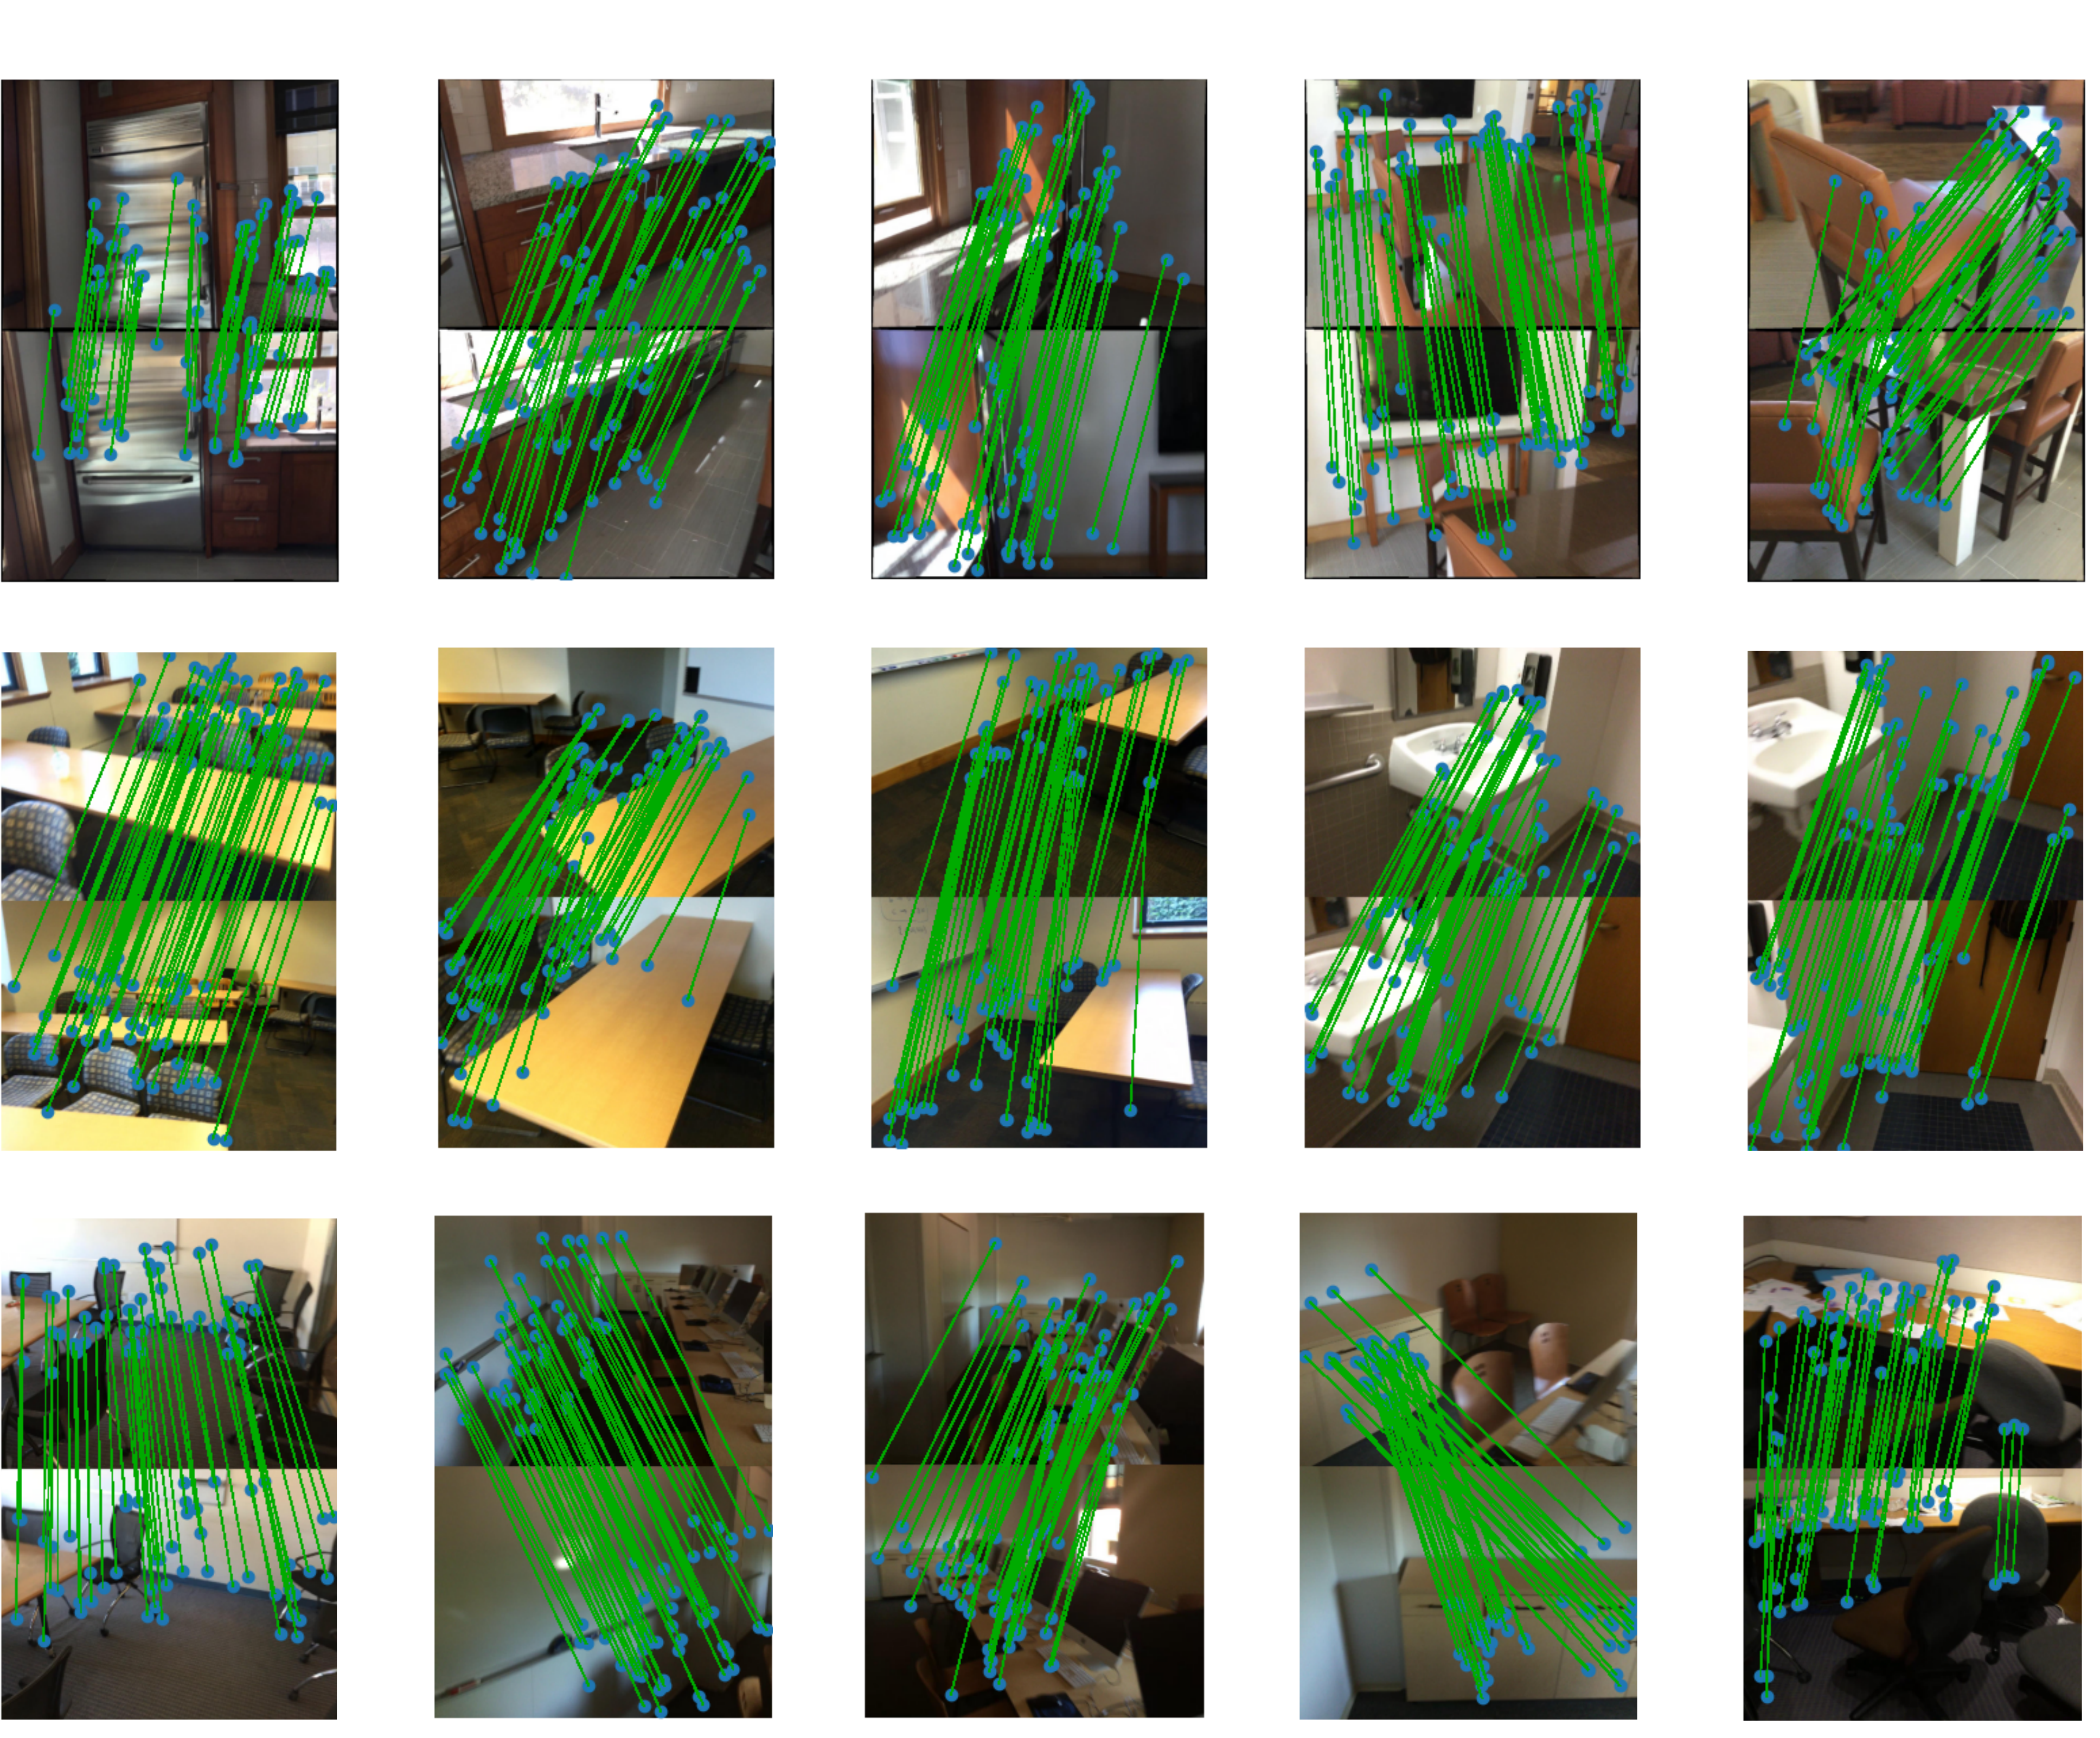}
    \end{center}
    \caption{\textbf{Qualitative results of multi-view consistency module prediction.} Each element consists of two different view images. The query points and prediction points are visualized using the blue dot, and they are connected by the green line.}
    \label{Fig:supp_cotr}
\end{figure}
