# Supplementary material for: Multi-View Representation is What You Need for Point-Cloud Pre-Training
Source: arXiv:2306.02558 source file (2024-04-28)
Supplement: Supplementary file 6 [file supp_radar_chart.tex]

\begin{figure}[h]
    \centering   
    \includegraphics[width=0.7\linewidth]{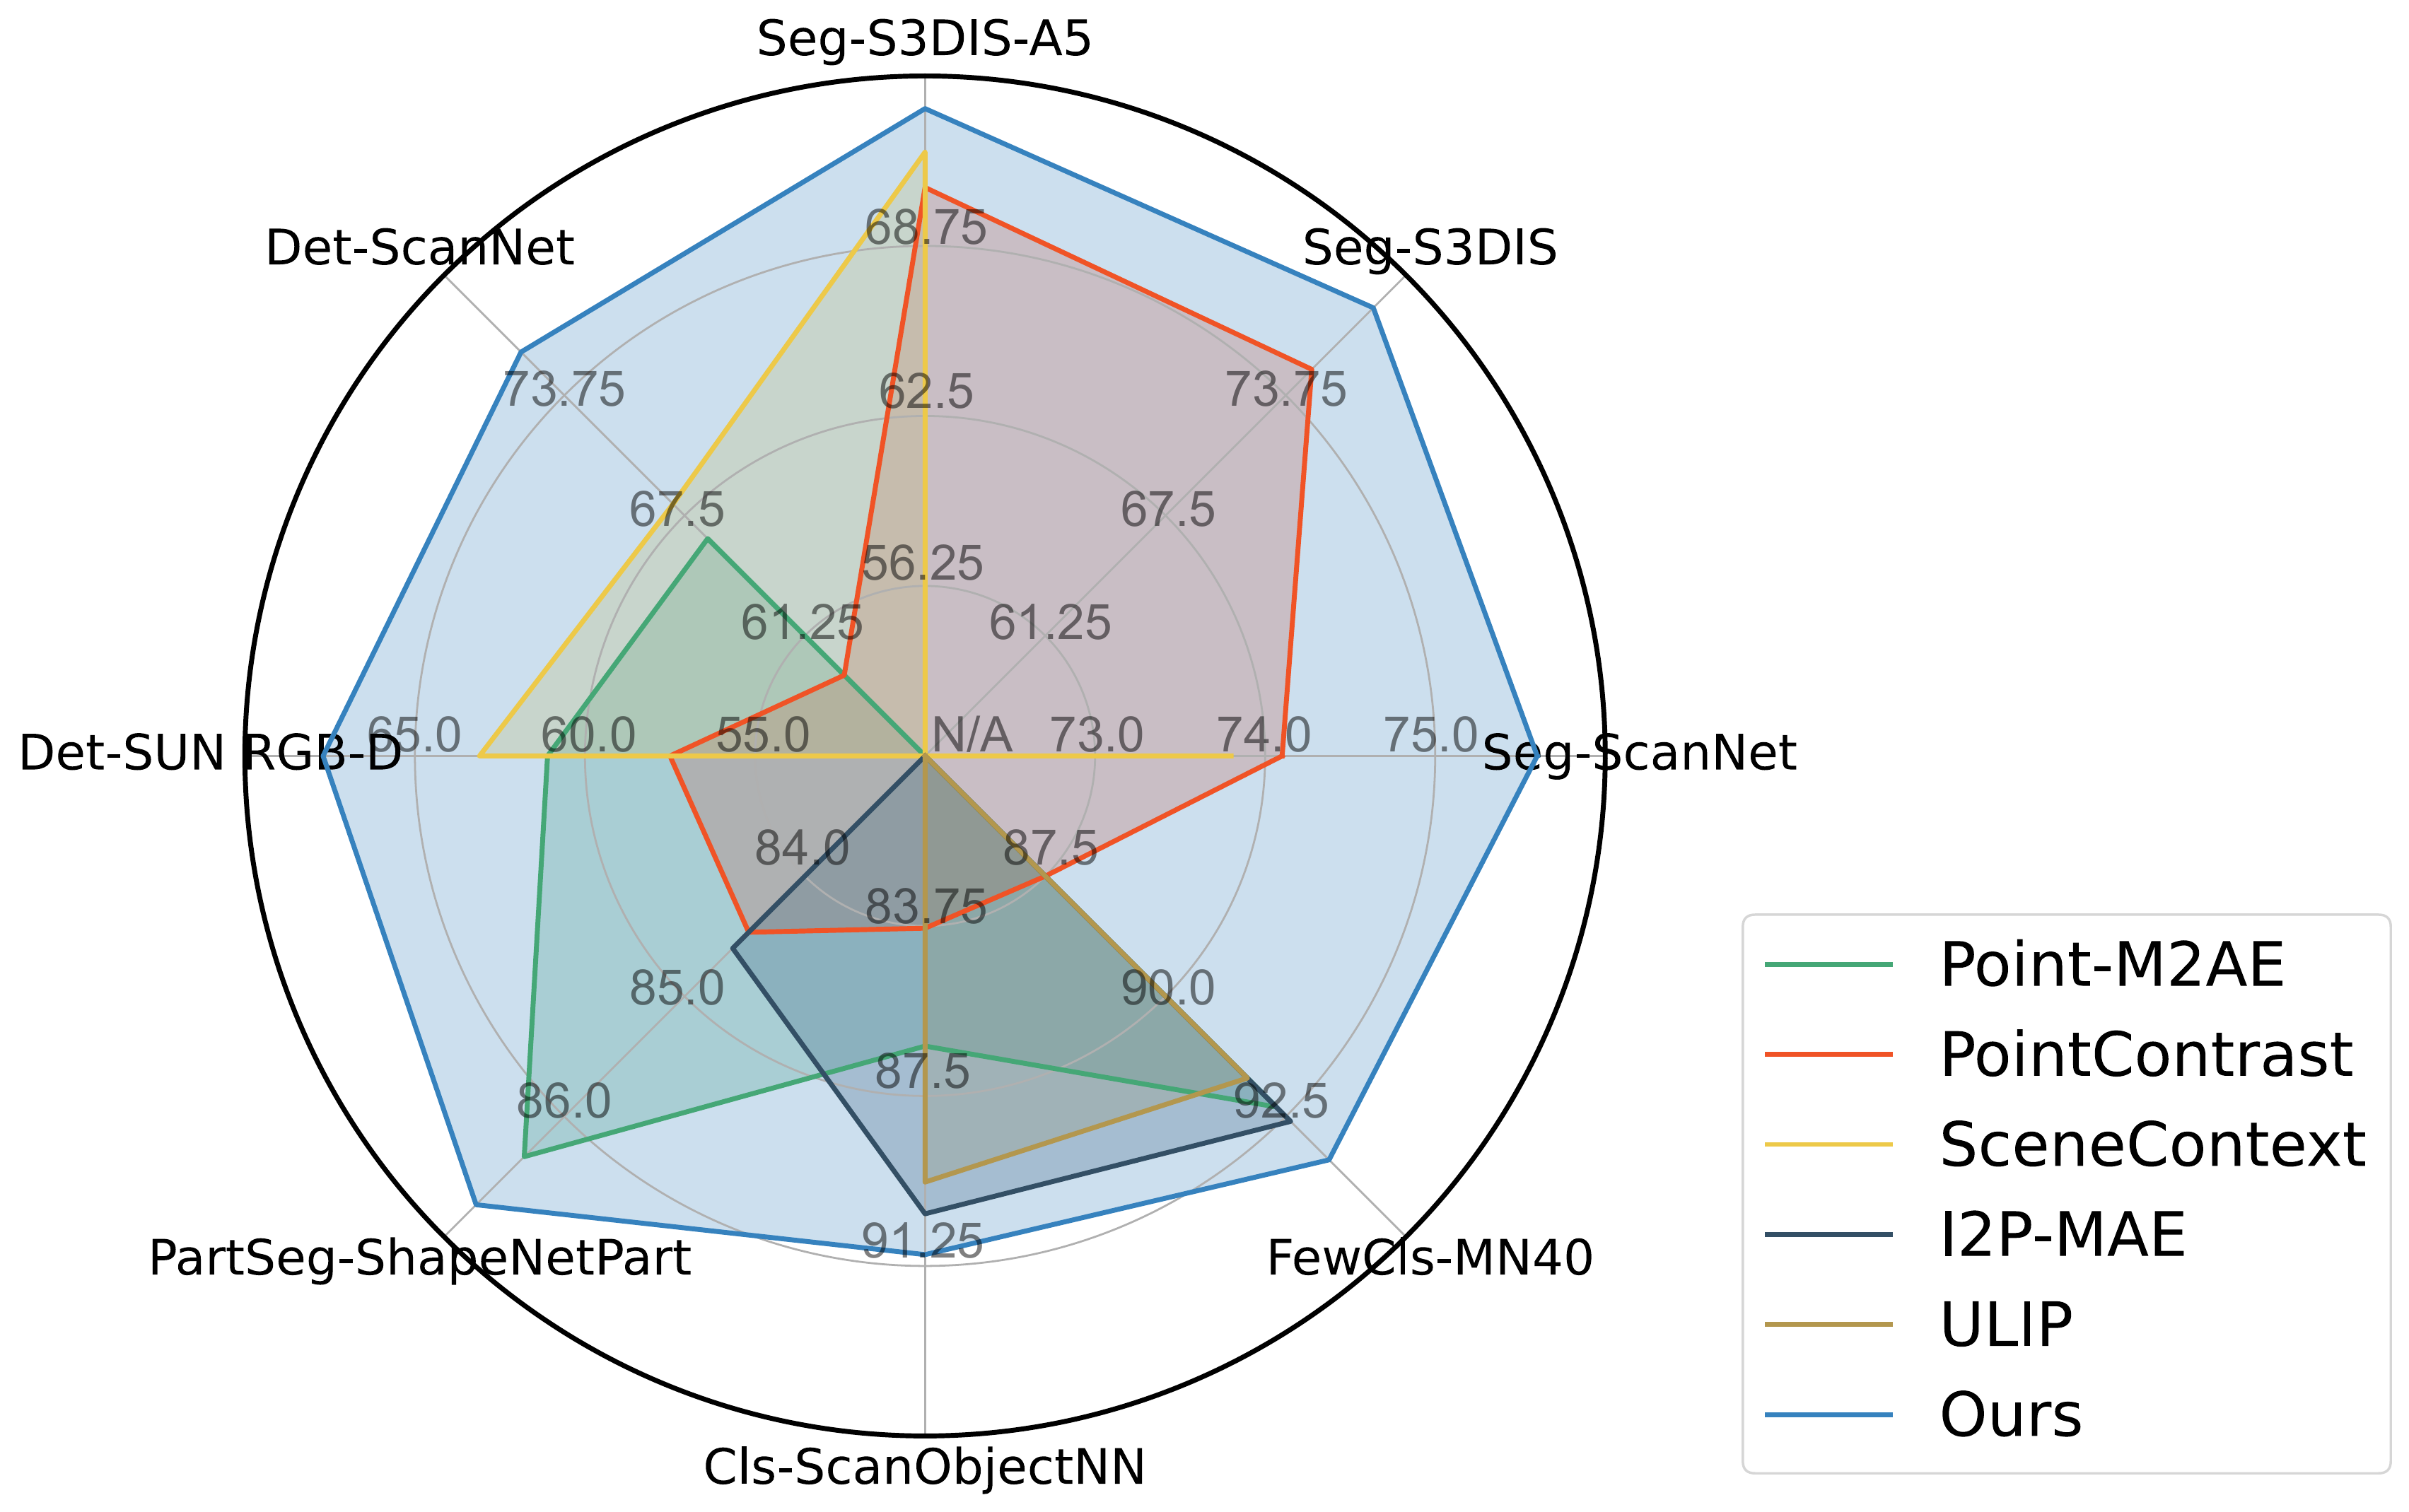}
    %\caption{Our model (blue) achieves state-of-the-art performance across a broad range of tasks at both the scene and shape levels. The distance to the origin indicates the task result.}
    \label{fig:radar}
\end{figure}
