# Supplementary material for: Multi-View Representation is What You Need for Point-Cloud Pre-Training
Source: arXiv:2306.02558 source file (2024-04-28)
Supplement: Supplementary file 7 [file supp_srnet.tex]

\begin{figure}[h]
    \begin{center}
    \includegraphics[width=1\linewidth]{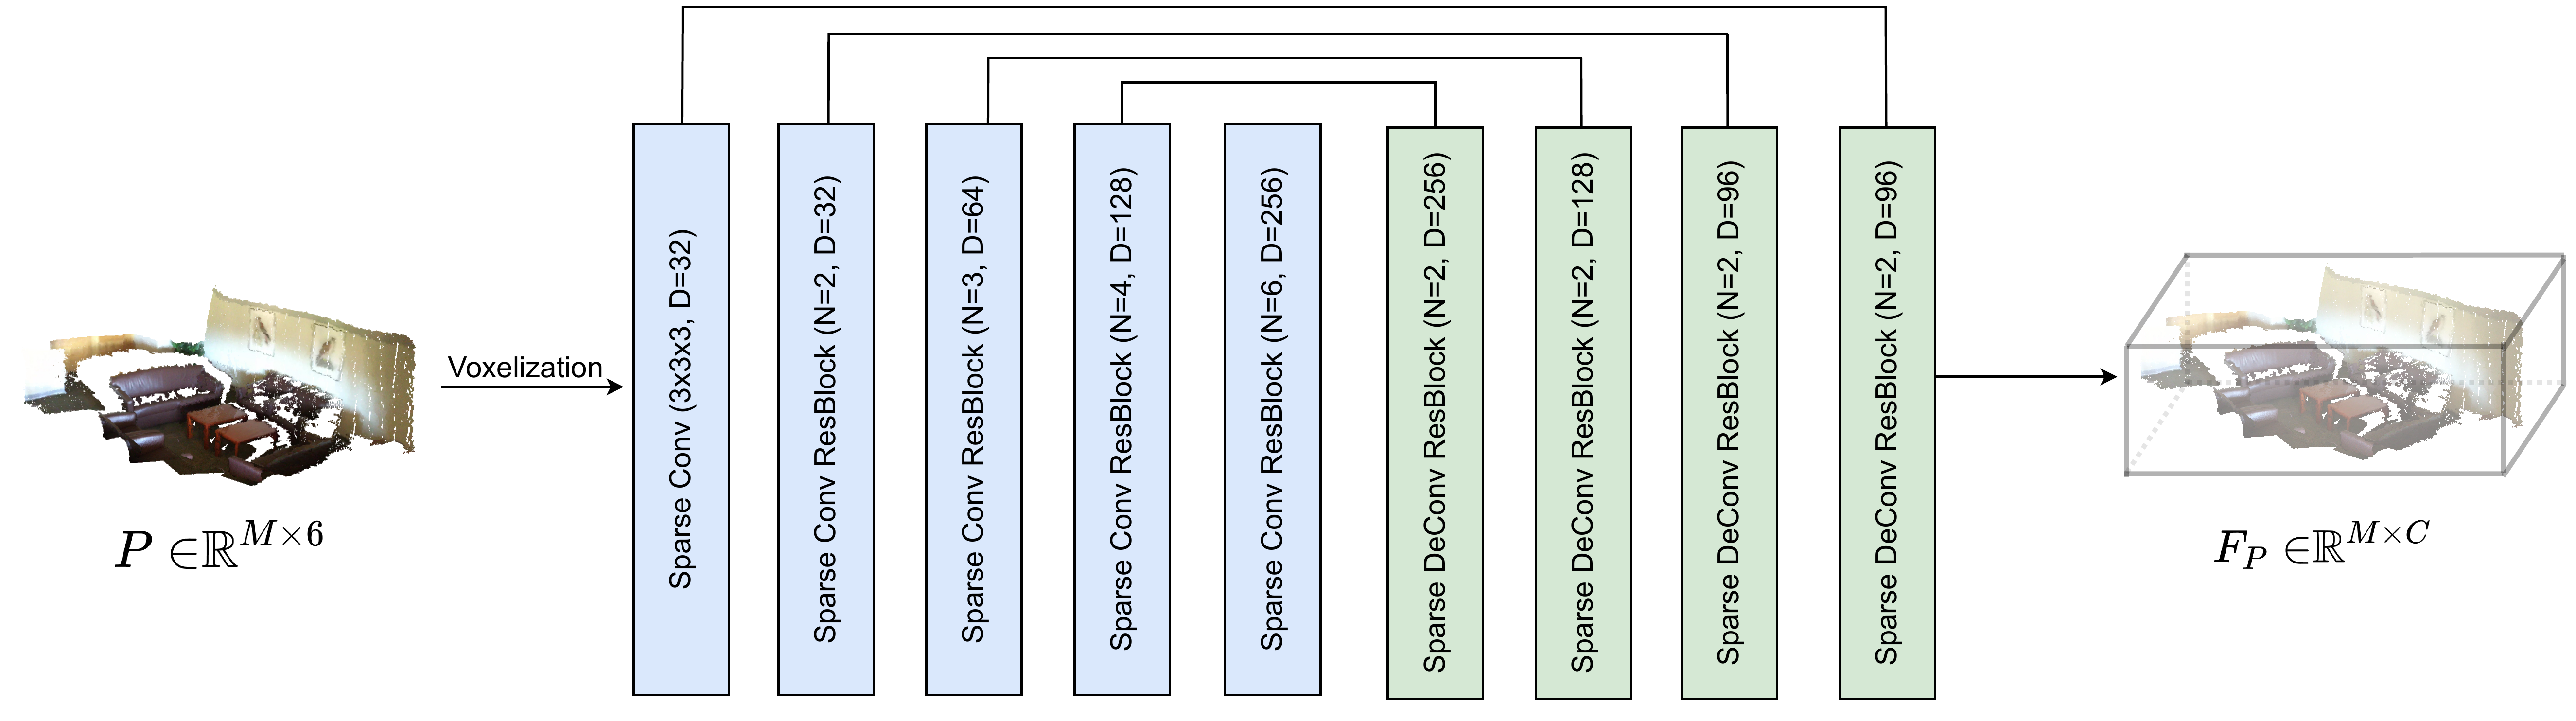}
    \end{center}
    \caption{\textbf{Feature encoding network details.}}
    \label{Fig:srnet}
\end{figure}
