# Supplementary material for: Multi-View Representation is What You Need for Point-Cloud Pre-Training
Source: arXiv:2306.02558 source file (2024-04-28)
Supplement: Supplementary file 9 [file supp_label_eff.tex]

\begin{table}[h]
\centering
\setlength\tabcolsep{8pt}
\begin{tabular}{lccc}
\toprule
\textbf{Method}            & \textbf{20\%} & \textbf{50\%} & \textbf{100\%} \\ 
\midrule
Train from scratch & 18.8          & 24.7          & 32.9           \\ 
PointContrast      & 24.5          & 29.2          & 37.5           \\ 
4DContrast         & 26.3          & 31.5          & 38.2           \\ 
MVNet              & \textbf{28.5} & \textbf{33.2} & \textbf{39.6}  \\ 
\bottomrule
\end{tabular}
\caption{\textbf{Label efficient training on SUN RGB-D object detection task.} We take the VoteNet as network architecture and compare our method with PointContrast and 4DContrast.}
\label{tab:supp-label}
\end{table}
